# Supplementary material for: AutoSynth: Learning to Generate 3D Training Data for Object Point Cloud Registration
Source: arXiv:2309.11170 source file (2023-09-20)
Supplement: Supplementary file 1 [file 6-supplementary.tex]

%\section{Appendix}
\section{Comparison of Models Trained on Different Datasets}
In addition to comparing the registration model trained on our data with that trained on the ModelNet40 dataset, here we provide results obtained by training on the ShapeNetCoreV2 dataset~\cite{Chang15}. ShapeNetCoreV2 is a synthetic dataset, as ModelNet40, but consisting of $57,448$ mesh models. We used the mesh models in its training split for training, $35,708$ meshes in total. Here, we use BPNet as registration model and evaluate its performance on the TUD-L dataset. In \cref{tab:syn_datasets}, we compare the performance of models trained on three different datasets: ModelNet40, ShapeNetCoreV2 and our AutoSynth searched dataset. The model trained on our AutoSynth searched dataset outperforms the other two. The model trained on ShapeNetCoreV2 achieves even worse results than the one trained on ModelNet40. This further evidences that simply increasing the number of models does not lead to a performance increase; both ShapeNetCoreV2 and ModelNet40 contain clean, manually-designed models, and thus do not yield a registration network that generalizes well to real data. By contrast, our data generation and search procedure is able to yield models that depict closer information to that in a real-scan dataset, resulting in higher performance.
%and diversity.
\begin{table}[!ht]
    \centering
    {% \scriptsize
    \setlength{\tabcolsep}{1.mm}{
    \begin{tabular}{l|ccc|ccc|c}
        \toprule
        & \multicolumn{3}{c|}{Rotation mAP} & \multicolumn{3}{c|}{Translation mAP} & \multicolumn{1}{c}{ADD} \\
        Method & $5^{\circ}$ & $10^{\circ}$ & $20^{\circ}$ & $1cm$ & $2cm$ & $5cm$ & $0.1d$ \\
        \midrule
        ShapeNetCoreV2      & 0.67 & 0.70 & 0.73 & 0.67 & 0.77 & 0.87 & 0.73 \\
        ModelNet40          & 0.71 & 0.74 & 0.77 & 0.70 & 0.80 & 0.94 & 0.76 \\
        AutoSynth           & 0.78 & 0.81 & 0.85 & 0.77 & 0.86 & 0.95 & 0.84 \\
        \bottomrule
    \end{tabular}
    }}
    \caption{Comparison of BPNet trained with different synthetic datasets and evaluated on the TUD-L dataset.}
    \label{tab:syn_datasets}
\end{table}

\section{Influence of Shape Diversity}
In addition to Table 4 in the main paper, which demonstrates the influence of shape diversity on registration performance on the TUD-L dataset, here, we  provide similar results on the LINEMOD and Occluded-LINEMOD dataset. As shown in \cref{tab:tendency_full}, both datasets exhibit the same trend as TUD-L as the number of training meshes changes. In short, increasing the number of training models improves registration accuracy and lowers reconstruction error. These results further support the validity of our argument. Notably, the results obtained with our AutoSynth searched dataset are the best on all three tested datasets, validating the higher diversity of our data and the effectiveness of our method.
\begin{table*}[!t]
    \centering
    {%\scriptsize
    \setlength{\tabcolsep}{2.67mm}{
    \begin{tabular}{l|c|ccc|ccc|c|cccc}
        \toprule
        & \multicolumn{1}{c|}{Method} & \multicolumn{7}{c|}{BPNet} & \multicolumn{1}{c}{AutoEncoder} \\
        \midrule
        \multicolumn{1}{c|}{} & & \multicolumn{3}{c|}{Rotation mAP} & \multicolumn{3}{c|}{Translation mAP} & \multicolumn{1}{c|}{ADD} & \multicolumn{1}{c}{Recontruction} \\
        \multicolumn{1}{c|}{Dataset} & \multicolumn{1}{c|}{Setting}  & $5^{\circ}$ & $10^{\circ}$ & $20^{\circ}$ & $1cm$ & $2cm$ & $5cm$ & $0.1d$ & Chamfer Dist\\
        \midrule
        \multirow{6}{*}{TUD-L} 
        & MN40(01\_per\_cate)         & 0.59 & 0.62 & 0.68 & 0.59 & 0.71 & 0.92 & 0.65 & 22.27 \\ % ckpt/SA_modelnet_01_per_category/ckpt_best.pth.tar
        & MN40(05\_per\_cate)         & 0.61 & 0.66 & 0.69 & 0.62 & 0.74 & 0.90 & 0.68 & 17.81 \\ 
        & MN40(10\_per\_cate)         & 0.66 & 0.70 & 0.73 & 0.66 & 0.82 & 0.92 & 0.72 & 9.97 \\ % ckpt/SA_modelnet_10_per_category_random/iter_41000.pth.tar
        & MN40(50\_per\_cate)         & 0.69 & 0.72 & 0.75 & 0.69 & 0.81 & 0.91 & 0.75 & 6.82 \\  % Latest
        & MN40-full                   & 0.71 & 0.74 & 0.77 & 0.70 & 0.80 & 0.94 & 0.76 & 6.65 \\
        & AutoSynth                      & 0.78 & 0.81 & 0.85 & 0.77 & 0.86 & 0.95 & 0.84 & 4.16  \\
        \midrule
        \multirow{6}{*}{LM} 
        & MN40(01\_per\_cate)        & 0.25 & 0.35 & 0.44 & 0.33 & 0.66 & 0.92 & 0.37 & 33.28 \\
        & MN40(05\_per\_cate)        & 0.27 & 0.38 & 0.46 & 0.35 & 0.68 & 0.94 & 0.39 & 26.01 \\
        & MN40(10\_per\_cate)        & 0.29 & 0.41 & 0.49 & 0.37 & 0.71 & 0.95 & 0.42 & 12.12 \\ 
        & MN40(50\_per\_cate)        & 0.31 & 0.43 & 0.52 & 0.37 & 0.69 & 0.94 & 0.44 & 9.83 \\ %latest
        & MN40-full                  & 0.31 & 0.42 & 0.50 & 0.37 & 0.69 & 0.95 & 0.43 & 9.59 \\
        & AutoSynth                     & 0.36 & 0.49 & 0.58 & 0.40 & 0.74 & 0.93 & 0.50 & 7.01 \\
        \midrule
        \multirow{6}{*}{LMO} 
        & MN40(01\_per\_cate)          & 0.12 & 0.19 & 0.23 & 0.21 & 0.57 & 0.87 & 0.21 & 31.54 \\
        & MN40(05\_per\_cate)          & 0.16 & 0.26 & 0.35 & 0.26 & 0.61 & 0.90 & 0.28 & 23.47 \\
        & MN40(10\_per\_cate)          & 0.20 & 0.29 & 0.36 & 0.29 & 0.60 & 0.91 & 0.29 & 11.58 \\
        & MN40(50\_per\_cate)          & 0.22 & 0.33 & 0.43 & 0.27 & 0.61 & 0.92 & 0.34 & 9.45 \\
        & MN40-full                    & 0.22 & 0.32 & 0.41 & 0.30 & 0.63 & 0.92 & 0.34 & 9.42 \\
        & AutoSynth                       & 0.25 & 0.35 & 0.41 & 0.34 & 0.65 & 0.92 & 0.37 & 6.43 \\
        \bottomrule
    \end{tabular}
    }}
    \caption{
    Quantitative comparison of BPNet trained with different dataset settings and evaluated on the \textbf{TUD-L, LINEMOD, and Occluded-LINEMOD} real scene datasets. For the ModelNet40, we pick 1, 5, 10 and 50 mesh models from each category, corresponding to 40, 200, 400, 2000 mesh models.
    The Chamfer distance is multiplied by $10^3$. Note that, for both registration and reconstruction, increasing the number of training mesh models improves the performance. 
    %\MS{If we need to save space, we could keep only one dataset here and move the other two to the supplementary materia.}
    }
    \label{tab:tendency_full}
    % \vspace{-2.25em}
\end{table*}
